# Supplementary material for: Long-Range Nematic Order in Two-Dimensional Active Matter
Source: arXiv:2104.05453 ancillary file (2021-04-12)
Supplement: Supplementary file 1 [file SUPP-LRO-nematics.pdf]

# Long-Range Nematic Order in Two-Dimensional Active Matter
# – Supplementary Material–

Benoît Mahault[1] and Hugues Chaté[2,3]

[1] Max Planck Institute for Dynamics and Self-Organization (MPIDS), 37077 Göttingen, Germany
[2] Service de Physique de l'Etat Condensé, CEA, CNRS Université Paris-Saclay, CEA-Saclay, 91191 Gif-sur-Yvette, France
[3] Computational Science Research Center, Beijing 100193, China

(Dated: April 12, 2021)

## DETAILS ABOUT NUMERICAL SIMULATIONS

Simulations of the Vicsek-style self propelled rods (Eqs. (1) of the main text) were carried out in two dimensional periodic domains of size $L^2$. For the data presented in Fig. 2 of the main text, $L$ is fixed to 8192 which for $\bar{\rho} = 2$ corresponds to large scale simulations involving more than $10^8$ particles, while averages were performed over $10^6$ to $10^7$ time steps. Considering smaller sizes, we moreover checked that our results on correlation functions are not subject to finite size effects and that the scaling regimes shown can be considered asymptotic. As discussed in Ref. [1], systems in periodic domains are subject to diffusion of the global order direction due to the rotational symmetry of the microscopic model. However, the corresponding diffusion coefficient decreases with system size leading to slower wandering of the order. For the anisotropic correlation function data shown in Fig. 2 of the main text, we checked that the deviations of the global order direction from its mean axis over the whole measurement window did not exceed $0.01\pi$.

For the data presented in Fig. 1 of the main text, the local slope of the order parameter decay with system size $\sigma(L)$ was defined for two consecutive system sizes $L_{n,n+1}$ as $\sigma(\sqrt{L_n L_{n+1}}) \equiv -\ln[S(L_{n+1})/S(L_n)]/\ln[L_{n+1}/L_n]$. Using the expected power law behavior $S(L) - S(\infty) \sim L^{-\varpi}$, one obtains

$$\sigma(L) = -\frac{\mathrm{d}\ln(S)}{\mathrm{d}\ln(L)} \sim \frac{\varpi L^{-\varpi}}{S(\infty) + \mathcal{O}(L^{-\varpi})}, \tag{1}$$

such that for $S(\infty) > 0$, which corresponds to long-range order, $\sigma(L) \sim L^{-\varpi}$ for $L \to \infty$, while in a quasi-ordered phase ($S(\infty) = 0$) $\sigma(L) = \varpi$.

## CONSTRUCTION OF THE BOLTZMANN EQUATION

In this section, we detail the construction of the Boltzmann equation from which the hydrodynamic theory of homogeneous nematic phase in the limit of slow reversals is derived. As motivated in the main text, we describe this phase as formed by two distinct populations, hereafter denoted $R$ and $L$, of polar active particles aligning their directions of motion polarly with neighbors if they belong to the same population, or anti-aligning it otherwise. The corresponding Vicsek-style microscopic rules for the evolution of the positions and orientations of the $L$ and $R$ particles are

$$\mathbf{r}_{i,L}^{t+1} = \mathbf{r}_{i,L}^{t} + v_0 \mathbf{e}_{i,L}^{t+1}, \qquad \mathbf{r}_{i,R}^{t+1} = \mathbf{r}_{i,R}^{t} + v_0 \mathbf{e}_{i,R}^{t+1}, \tag{2a}$$

$$\mathbf{e}_{i,L}^{t+1} = (\mathcal{R}_\eta \circ \vartheta)\, \langle \mathbf{e}_{j,L}^{t} - \mathbf{e}_{j,R}^{t} \rangle_{j\sim i}, \qquad \mathbf{e}_{i,R}^{t+1} = (\mathcal{R}_\eta \circ \vartheta)\, \langle \mathbf{e}_{j,R}^{t} - \mathbf{e}_{j,L}^{t} \rangle_{j\sim i}, \tag{2b}$$

where $v_0$ denotes the constant self-propulsion speed and the operators $\mathcal{R}_\eta$ and $\vartheta$ are defined in the main text.

Following the standard Boltzmann-Ginzburg-Landau (BGL) approach [2, 3], the Boltzmann equations describing Eqs. (2) take the rather generic form:

$$\partial_t f_R + v_0 \boldsymbol{e}(\theta) \cdot \nabla f_R = \tau_r^{-1} (f_L - f_R) + I_{\rm sd}[f_R] + I_{\rm co}[f_R, f_L]\ , \tag{3a}$$

$$\partial_t f_L + v_0 \boldsymbol{e}(\theta) \cdot \nabla f_L = \tau_r^{-1} (f_R - f_L) + I_{\rm sd}[f_L] + I_{\rm co}[f_L, f_R]\ , \tag{3b}$$

where $f_{R/L}(\boldsymbol{r}, \theta, t)$ denote the single particle distributions associated with populations $R$ and $L$, $\theta$ parametrizes velocity orientations, and $\tau_r^{-1} (= \ell_r/v_0)$ is the typical switching rate between populations $R$ and $L$. The self-diffusion integral $I_{\rm sd}$ describes the effect of orientational noise characterized by the distribution $P(\theta)$. In order to account for

the discrete time Vicsek-style dynamics, we model orientational diffusion as resulting from tumbling events occurring at rate $\lambda$, hence

$$I_{\rm sd}\left[f\right] = \lambda\left[-f(\boldsymbol{r},\theta,t) + \int \mathrm{d}\theta' f(\boldsymbol{r},\theta',t) P(\theta-\theta')\right] . \tag{4}$$

$I_{\rm co}$ describes the evolution of the distributions due to collision events. As usually done in this context, we assume the collisions to be binary (dilute limit) and local, and moreover work under the molecular chaos hypothesis, such that

$$\begin{aligned} I_{\rm co}\left[f_1,f_2\right] = & -f_1(\boldsymbol{r},\theta,t)\int \mathrm{d}\theta'\, K(\theta'-\theta)\left[f_1(\boldsymbol{r},\theta',t)+f_2(\boldsymbol{r},\theta',t)\right] \\ & + \int \mathrm{d}\theta_1 \mathrm{d}\theta_2\, f_1(\boldsymbol{r},\theta_1,t)K(\theta_2-\theta_1)\Big[f_1(\boldsymbol{r},\theta_2,t)P(\theta-\Psi_{\rm p}(\theta_1,\theta_2)) + f_2(\boldsymbol{r},\theta_2,t)P(\theta-\Psi_{\rm ap}(\theta_1,\theta_2))\Big] . \end{aligned} \tag{5}$$

Here for simplicity we consider identical noise distributions for the collisional and self-diffusion integrals. Eq. (5) depends on three quantities. First, the Kernel of interaction $K(\Delta)$ is set by the symmetry of the particle's motion, and in this case without explicit reversals is given by [2]

$$K(\Delta) = 4r_0 v_0 \left|\sin\left(\frac{\Delta}{2}\right)\right| , \tag{6}$$

with $r_0$ denoting the radius of interaction. Secondly, $\Psi_{\rm p}(\theta_1,\theta_2)$ and $\Psi_{\rm ap}(\theta_1,\theta_2)$ define the alignment rule respectively between particles 1 and 2 belonging to the same and different populations. From the rotational invariance of the problem, we can write them as $\Psi_{\rm p,ap}(\theta_1,\theta_2) = \theta_1 + H_{\rm p,ap}(\theta_2-\theta_1)$, while given the microscopic rules of Eqs. (2) the $H$ functions are $2\pi$-periodic and read

$$\theta_1 + H_{\rm p}(\theta_2-\theta_1) = \mathrm{Arg}\left[e^{i\theta_1}+e^{i\theta_2}\right] = \theta_1 + \frac{\theta_2-\theta_1}{2} \qquad \text{for} \quad -\pi < \theta_2-\theta_1 \le \pi , \tag{7a}$$

$$\theta_1 + H_{\rm ap}(\theta_2-\theta_1) = \mathrm{Arg}\left[e^{i\theta_1}-e^{i\theta_2}\right] = \theta_1 + \frac{\theta_2-\theta_1-\pi}{2} + \pi\Theta(\theta_1-\theta_2) \qquad \text{for} \quad -\pi < \theta_2-\theta_1 \le \pi , \tag{7b}$$

where Arg$[z]$ returns the argument of the complex number $z$ and $\Theta$ is the Heaviside function.

To simplify the notations, in the following we work with non-dimensional quantities such that we apply the rescalings:

$$t \to t/\lambda, \qquad \boldsymbol{r} \to v_0\boldsymbol{r}/\lambda, \qquad \tau_r \to \tau_r/\lambda, \qquad f^{R/L} \to \lambda f^{R/L}/(2r_0v_0) . \tag{8}$$

Following the BGL approach, we now expand $f_{R/L}$ and $P$ into Fourier series: $f_{R/L}(\boldsymbol{r},\theta,t) = \frac{1}{2\pi}\sum_k f_k^{R/L}(\boldsymbol{r},t)\exp(-ik\theta)$, $P(\theta) = \frac{1}{2\pi}\sum_k P_k \exp(-ik\theta)$, and rewrite Eqs. (3) as

$$\begin{aligned} \partial_t f_k^{R/L} + \frac{1}{2}\left(\nabla^* f_{k+1}^{R/L} + \nabla f_{k-1}^{R/L}\right) = & \ \tau_r^{-1}\left(f_k^{L/R} - f_k^{R/L}\right) + (P_k-1) f_k^{R/L} \\ & + \sum_{q=-\infty}^{\infty} f_{k-q}^{R/L}\left[P_k\left(I_{k,q}^{\rm p} f_q^{R/L} + I_{k,q}^{\rm ap} f_q^{L/R}\right) - I_{0,q}(f_q^{R/L}+f_q^{L/R})\right] , \end{aligned} \tag{9}$$

where $P_k$ are the Fourier modes of $P$, $\nabla \equiv \partial_x + i\partial_y$ denotes the complex gradient, and

$$I_{k,q}^{\rm p} \equiv \frac{1}{\pi}\int_{-\pi}^{\pi}\mathrm{d}\Delta \left|\sin\left(\frac{\Delta}{2}\right)\right| e^{ikH_{\rm p}(\Delta)-iq\Delta} = \frac{4}{\pi}\frac{1+(-1)^q\sin\left(\frac{\pi k}{2}\right)(k-2q)}{1-(k-2q)^2} \left(= \frac{2}{\pi} \text{ if } k-2q = \pm 1\right) ,$$

$$I_{k,q}^{\rm ap} \equiv \frac{1}{\pi}\int_{-\pi}^{\pi}\mathrm{d}\Delta \left|\sin\left(\frac{\Delta}{2}\right)\right| e^{ikH_{\rm ap}(\Delta)-iq\Delta} = \frac{4}{\pi}\frac{\cos\left(\frac{\pi k}{2}\right)}{1-(k-2q)^2} \left(= (-1)^q \text{ if } k-2q = \pm 1\right) ,$$

such that $I_{0,q}^{\rm p} = I_{0,q}^{\rm ap} \equiv I_{0,q}$ and it appears clearly that all coefficients of the nonlinear terms in Eq. (9) are real.

As we will show below, the fields

$$f_k \equiv f_k^R + f_k^L , \qquad g_k \equiv f_k^R - f_k^L , \tag{10}$$

directly relate to physical quantities and are thus more convenient to deal with. For instance, $\rho \equiv f_0$ is the total particle density, while $g_0$ measures local differences in the densities of $R$ and $L$ particles. Similarly, $f_1$ is the total

polar field while $g_1$ can be seen as a measure of the polar order within each populations: for a perfectly aligned system with equal densities of $R$ and $L$ particles pointing respectively towards $\theta = 0$ and $\pi$, $f_1 = 0$ while $g_1 > 0$.

Using this new definition of the modes, from Eq. (9) we get

$$\partial_t f_k + \frac{1}{2}\left(\nabla^* f_{k+1} + \nabla f_{k-1}\right) = (P_k - 1) f_k + \sum_q J_{k,q} f_q f_{k-q} + L_{k,q} g_q g_{k-q}\,, \tag{11a}$$

$$\partial_t g_k + \frac{1}{2}\left(\nabla^* g_{k+1} + \nabla g_{k-1}\right) = \left(P_k - 1 - 2\tau_r^{-1}\right) g_k + \sum_q \left(L_{k,q} + J_{k,k-q}\right) g_q f_{k-q}\,, \tag{11b}$$

where we have defined

$$J_{k,q} \equiv \frac{P_k}{2}\left(I^{\rm p}_{k,q} + I^{\rm ap}_{k,q}\right) - I_{0,q}, \qquad L_{k,q} \equiv \frac{P_k}{2}\left(I^{\rm p}_{k,q} - I^{\rm ap}_{k,q}\right)\,.$$

## TRUNCATION AND CLOSURE, DERIVATION OF THE HYDRODYNAMIC EQUATIONS

We now present the systematic procedure we use to truncate and close the hierarchy (11) so as to obtain hydrodynamic equations valid close to the onset of order in the large-scale and long time limits. We consider a homogeneous disordered system with mean density $\rho = \bar\rho$ and equal densities of $R$ and $L$ particles ($g_0 = 0$). Little uniform perturbations around that state thus follow for $k > 0$

$$\partial_t \delta f_k = \mu_k[\bar\rho]\delta f_k, \qquad \partial_t \delta g_k = \nu_k[\bar\rho]\delta g_k\,, \tag{12}$$

while $\partial_t \delta g_0 = -2\tau_r^{-1}\delta g_0$. Here, we have defined the linear coefficients

$$\mu_k[\bar\rho] \equiv P_k - 1 + (J_{k,0} + J_{k,k})\bar\rho, \qquad \nu_k[\bar\rho] \equiv P_k - 1 - 2\tau_r^{-1} + (J_{k,0} + L_{k,k})\bar\rho\,, \tag{13}$$

which for the first values of $k$ read

$$\mu_1[\bar\rho] = P_1 - 1 + \frac{2(3P_1 - 4)\bar\rho}{3\pi} \quad (<0)\,, \qquad \nu_1[\bar\rho] = P_1 - 1 - 2\tau_r^{-1} + \frac{((2+\pi)P_1 - 4)\bar\rho}{\pi}\,,$$

$$\mu_2[\bar\rho] = P_2 - 1 - \frac{56\bar\rho}{15\pi} \quad (<0)\,, \qquad \nu_2[\bar\rho] = P_2 - 1 - 2\tau_r^{-1} - \frac{4(P_2+3)\bar\rho}{3\pi} \quad (<0)\,,$$

$$\mu_3[\bar\rho] = P_3 - 1 - \frac{2(35P_3 + 68)\bar\rho}{35\pi} \quad (<0)\,, \qquad \nu_3[\bar\rho] = P_3 - 1 - 2\tau_r^{-1} - \frac{2(P_3+2)\bar\rho}{\pi} \quad (<0)\,,$$

$$\ldots$$

Therefore, for $\bar\rho > \pi(1 - P_1 + 2\tau_r^{-1})/((2+\pi)P_1 - 4)$ the growth rate of the perturbation $\delta g_1$ is positive, leading the disordered homogeneous solution to be linearly unstable. Note that here $\mu_2[\bar\rho]$ is always negative, contrary to what is found in the usual treatment of active nematics [2, 4]. This comes from our particular choice of interactions, which in the homogeneous ordered phase give rise to overall nematic order (actually, $f_2$ is expect to be eventually nonzero due to the nonlinear coupling with $g_1$), but are generally not equivalent to nematic alignment. Indeed, since we consider here interactions that are $2\pi-$periodic, two particles from different populations will anti-align even if their orientations initially form an acute angle.

The BGL approach offers a controlled procedure to truncate and close the hierarchy of modes by assuming the ordering field to be small, therefore close to the onset of order we set $|g_1| \sim \varepsilon \ll \bar\rho$. Inspecting the leading order nonlinear terms of Eq. (11a), we find

$$|f_k| \sim |g_1 g_{k-1}| \qquad (k \geq 1)\,, \tag{14a}$$

while the symmetry of the motion imposes the ballistic scaling $\partial_t \sim \nabla \sim \varepsilon$ such that the dominant contribution to the $g_k$ modes is

$$|g_k| \sim |\nabla g_{k-1}| \qquad (k > 1)\,. \tag{14b}$$

From the exact equations for the density $\rho$ and $g_0$,

$$\partial_t \rho = -\mathrm{Re}\left[\nabla^* f_1\right]\,, \tag{15a}$$

$$\partial_t g_0 = -2\tau_r^{-1} g_0 - \mathrm{Re}\left[\nabla^* g_1\right] , \tag{15b}$$

we moreover find that density fluctuations obey $|\rho - \bar{\rho}| \equiv |\delta\rho| \sim |f_1|$, while $|g_0| \sim |g_1|$ is obtained in the limit of arbitrary large $\tau_r$. Overall, we thus have

$$|g_0| \sim \varepsilon\,, \quad |g_{k\geq 1}| \sim \varepsilon^k\,, \quad |\delta\rho| \sim |f_1| \sim \varepsilon^2, \quad |f_{k>1}| \sim \varepsilon^k, \quad \partial_t \sim \nabla \sim \varepsilon\,. \tag{16}$$

For $(k > 0)$, the hierarchy truncated up to order $\varepsilon^4$ reads

$$\partial_t f_1 = -\frac{1}{2}\left(\nabla^* f_2 + \nabla\rho\right) + \mu_1[\rho] f_1 + (L_{1,0} + L_{1,1}) g_0 g_1 + (L_{1,-1} + L_{1,2}) g_1^* g_2 + (J_{1,-1} + J_{1,2}) f_1^* f_2 + \mathcal{O}(\varepsilon^5)\,, \tag{17a}$$

$$\partial_t g_1 = -\frac{1}{2}\left(\nabla^* g_2 + \nabla g_0\right) + \nu_1[\rho] g_1 + (L_{1,0} + J_{1,1}) g_0 f_1 + (L_{1,-1} + J_{1,2}) g_1^* f_2 + (L_{1,2} + J_{1,-1}) f_1^* g_2 + \mathcal{O}(\varepsilon^5)\,, \tag{17b}$$

$$\partial_t f_2 = -\frac{1}{2}\left(\nabla^* f_3 + \nabla f_1\right) + \mu_2[\rho] f_2 + (L_{2,0} + L_{2,2}) g_0 g_2 + L_{2,1} g_1^2 + J_{2,1} f_1^2 + (L_{2,3} + L_{2,-1}) g_1^* g_3 + \mathcal{O}(\varepsilon^6)\,, \tag{17c}$$

$$\partial_t g_2 = -\frac{1}{2}\left(\nabla^* g_3 + \nabla g_1\right) + \nu_2[\rho] g_2 + (L_{2,0} + J_{2,2}) g_0 f_2 + (L_{2,1} + J_{2,1}) g_1 f_1 + (L_{2,-1} + J_{2,3}) g_1^* f_3 + \mathcal{O}(\varepsilon^6)\,, \tag{17d}$$

$$\ldots$$

As $f_2$ and $g_2$ appear in the equations for $f_1$ and $g_1$ in terms of order at least $\varepsilon^3$, we neglect the terms of order $\varepsilon^4$ in Eqs. (17c) and (17d). This allows to neglect all terms involving $f_3$ and $g_3$, and therefore to express $f_2$ and $g_2$ (after setting $\partial_t f_2 = \partial_t g_2 = 0$) as

$$f_2 = \frac{\nabla f_1}{2\mu_2[\bar{\rho}]} - \frac{g_1^2}{\mu_2[\rho]} - \frac{(L_{2,0} + L_{2,2}) g_0}{2\mu_2[\bar{\rho}]\nu_2[\bar{\rho}]}\nabla g_1 + \mathcal{O}(\varepsilon^4)\,,$$

$$g_2 = \frac{\nabla g_1}{2\nu_2[\rho]} - \frac{(L_{2,1} + J_{2,1})}{\nu_2[\bar{\rho}]} g_1 f_1 + \frac{(L_{2,0} + J_{2,2}) g_0}{\mu_2[\bar{\rho}]\nu_2[\bar{\rho}]} g_1^2 + \mathcal{O}(\varepsilon^4)\,.$$

After replacing these expressions in the equations for $f_1$ and $g_1$, we obtain the closed hydrodynamic equations

$$\partial_t \rho = -\mathrm{Re}\left[\nabla^* f_1\right] , \tag{18a}$$

$$\partial_t g_0 = -2\tau_r^{-1} g_0 - \mathrm{Re}\left[\nabla^* g_1\right] , \tag{18b}$$

$$\partial_t f_1 = -\frac{1}{2}\nabla\rho + \left(\mu[\rho] - \xi|g_1|^2\right) f_1 + \left(\alpha[g_0] - \chi_1 g_0 |g_1|^2 - \chi_2 f_1^* g_1\right) g_1 + D_f \Delta f_1 + D_g g_0 \Delta g_1 + \kappa_1[\rho]\nabla^* g_1^2 + \kappa_2[\rho] g_1^* \nabla g_1 + \kappa_3 (\nabla^* g_0)(\nabla g_1)\,, \tag{18c}$$

$$\partial_t g_1 = -\frac{1}{2}\nabla g_0 - \sigma g_1^2 \nabla^* g_0 + \left(\nu[\rho] - \Gamma[\rho]|g_1|^2\right) g_1 + \beta[g_0] f_1 + \Omega[\rho]\Delta g_1 + \lambda_1 g_0 \nabla^* g_1^2 + \lambda_2 g_0 g_1^* \nabla g_1 + \lambda_3 g_1^* \nabla f_1 + \lambda_4 \nabla^*(g_1 f_1) + \lambda_5 f_1^* \nabla g_1\,, \tag{18d}$$

where $\mu[\rho] \equiv \mu_1[\rho]$, $\nu[\rho] \equiv \nu_1[\rho]$ and the other coefficients are given by

$$\xi \equiv \frac{8P_1(3P_2 + 1)}{\pi(4(P_2 + 3)\bar{\rho} + 3\pi(1 - P_2 + 2\tau_r^{-1}))}\ (> 0), \qquad \alpha[g_0] \equiv \frac{2P_1 g_0}{\pi},$$

$$\chi_1 \equiv \frac{-240 P_1 P_2}{(15\pi(1 - P_2) + 56\bar{\rho})(3\pi(1 - P_2 + 2\tau_r^{-1}) + 4(P_2 + 3)\bar{\rho})}\ (< 0), \qquad \chi_2 \equiv \frac{24(5P_1 - 4)P_2}{\pi(15\pi(1 - P_2) + 56\bar{\rho})},$$

$$D_g \equiv \frac{-30\pi P_2}{(15\pi(1 - P_2) + 56\bar{\rho})(3\pi(1 - P_2 + 2\tau_r^{-1}) + 4(P_2 + 3)\bar{\rho})}\ (< 0), \qquad D_f \equiv \frac{15\pi}{224\bar{\rho} + 60\pi(1 - P_2)}\ (> 0),$$

$$\kappa_1[\rho] \equiv \frac{-30P_2}{15\pi(1 - P_2) + 56\rho}\ (< 0), \qquad \kappa_2[\rho] \equiv \frac{3P_1}{4(P_2 + 3)\rho + 3\pi(1 - P_2 + 2\tau_r^{-1})}\ (> 0),$$

$$\kappa_3 = D_2,$$

$$\sigma \equiv \frac{-6\pi(5P_2 - 1)}{(15\pi(1 - P_2) + 56\bar{\rho})(3\pi(1 - P_2 + 2\tau_r^{-1}) + 4(P_2 + 3)\bar{\rho})}, \qquad \beta[g_0] \equiv \frac{(4 - 3(\pi - 2)P_1)g_0}{3\pi},$$

$$\Gamma[\rho] \equiv \frac{8(15P_1 - 2)P_2}{\pi(15\pi(1 - P_2) + 56\rho)}\ (> 0), \qquad \Omega[\rho] \equiv \frac{3\pi}{4(4(P_2 + 3)\rho + 3\pi(1 - P_2 + 2\tau_r^{-1}))}\ (> 0),$$

$$\lambda_2 \equiv \frac{8(2 - 15P_1)P_2}{(15\pi(1 - P_2) + 56\bar{\rho})(3\pi(1 - P_2 + 2\tau_r^{-1}) + 4(P_2 + 3)\bar{\rho})} \qquad \lambda_1 \equiv -\sigma,$$

$$\lambda_3 \equiv \frac{(15P_1-2)}{15\pi(1-P_2)+56\rho}\ (>0). \qquad \lambda_4 \equiv \frac{-2(3P_2+1)}{4(P_2+3)\bar\rho+3\pi(1-P_2+2\tau_r^{-1})}\ (<0),$$
$$\lambda_5 \equiv \frac{(3P_1-2)}{4(P_2+3)\bar\rho+3\pi(1-P_2+2\tau_r^{-1})}.$$

Eqs. (18) possess a structure qualitatively different than that usually found in hydrodynamic theories written for active nematics. Indeed, because of the $2\pi$-symmetry of the interaction between the particles, as well as their polar motion, the pairs of hydrodynamic equations derived above for resp. $(\rho, f_1)$ and $(g_0, g_1)$ resemble two coupled Toner-Tu equations [5] that describe dry polar active system. Both density and $g_0$ and advected by the corresponding order fields, which are $2\pi$-symmetric. The resulting equations are thus not invariant by space inversion: $\boldsymbol{x} \leftrightarrow -\boldsymbol{x}$ as it would be the case if mass transport was purely diffusive. As stated in the main text, discarding the couplings to $\rho$ and $f_1$, Eqs. (18b) and (18d) are *almost* like the Toner Tu equations in the limit $\tau_r \to \infty$. The missing terms $\sim g_0 g_1$ and $\sim g_1 \nabla g_1$ are however forbidden by the $R \leftrightarrow L$ symmetry of the problem, which imposes the equations to be invariant under $g \leftrightarrow -g$.

We now note that, although Eqs. (18) were formally derived at the onset of order (for small $\varepsilon$ values), the BGL approach has been shown to lead to qualitatively faithful results even outside its range of formal validity [2, 3]. By construction, it moreover provides hydrodynamic equations with a structure reflecting the symmetries of the problem, which is the crucial point for the following analysis focusing on universal properties of the fluctuating ordered phase.

Finally, the existing literature about the BGL method usually prescribes a truncation at order $\varepsilon^3$ [2, 3, 6] (see, however, [7]), while in the above we considered terms up to $\varepsilon^4$. As we will show in the following, the reason for this difference is due to the fact that in the case considered here density is not directly advected by order, leading to $\delta\rho \sim \varepsilon^2$. Therefore, getting the pressure term $\sim \nabla^2\rho$ in the equation for $g_1$ fluctuations after enslaving the fast fields (see the following section) requires to derive Eqs. (18) up to order $\varepsilon^4$.

## LINEAR PERTURBATIONS AROUND THE ORDERED PHASE

In this section we investigate the fate of linear perturbations around the homogeneous ordered solution of Eqs. (18) and derive the Fourier space expression of the correlation functions presented in the main text. Eqs. (18) admit a homogeneous ordered solution that satisfies

$$\rho = \bar\rho, \qquad g_0 = 0, \qquad f_1 = 0, \qquad g_1 = \bar g \equiv \sqrt{\nu[\bar\rho]/\Gamma[\bar\rho]}\,. \tag{19}$$

Here, without loss of generality, we have fixed the 'phase' of the complex number $\bar g$ to zero which amounts to choosing the homogeneous order along the $x$ direction. Separating the perturbations along ($\|$) and transverse ($\perp$) to the order $\delta f_1 = \delta f_\| + i\delta f_\perp$, $\delta g_1 = \delta g_\| + i\delta g_\perp$ and rewriting $\nabla = \partial_\| + i\partial_\perp$ we then get

$$\partial_t\delta\rho = -\partial_\|\delta f_\| - \partial_\perp\delta f_\perp\,, \tag{20a}$$
$$\partial_t\delta g_0 = -2\tau_r^{-1}\delta g_0 - \partial_\|\delta g_\| - \partial_\perp\delta g_\perp\,, \tag{20b}$$
$$\partial_t\delta f_\| = -\frac{1}{2}\partial_\|\delta\rho - \zeta_\|\delta f_\| + \bar g\left(\partial\alpha - \chi_1\bar g^2\right)\delta g_0 + D_f\Delta\delta f_\| + \kappa_+\bar g\partial_\|\delta g_\| + \kappa_-\bar g\partial_\perp\delta g_\perp\,, \tag{20c}$$
$$\partial_t\delta f_\perp = -\frac{1}{2}\partial_\perp\delta\rho - \zeta_\perp\delta f_\perp + D_f\Delta\delta f_\perp + \kappa_+\bar g\partial_\|\delta g_\perp - \kappa_-\bar g\partial_\perp\delta g_\|\,, \tag{20d}$$
$$\partial_t\delta g_\| = -\left(\frac{1}{2} + \sigma\bar g^2\right)\partial_\|\delta g_0 - 2\nu[\bar\rho]\delta g_\| + \bar g\left(\partial\nu - \partial\Gamma\bar g^2\right)\delta\rho + \Omega[\bar\rho]\Delta\delta g_\| + \lambda_+\bar g\partial_\|\delta f_\| + \lambda_-\bar g\partial_\perp\delta f_\perp\,, \tag{20e}$$
$$\partial_t\delta g_\perp = -\left(\frac{1}{2} - \sigma\bar g^2\right)\partial_\perp\delta g_0 + \Omega[\bar\rho]\Delta\delta g_\perp + \lambda_+\bar g\partial_\|\delta f_\perp - \lambda_-\bar g\partial_\perp\delta f_\|\,, \tag{20f}$$

where we have defined $\partial\alpha \equiv \mathrm{d}\alpha/\mathrm{d}g_0$, $\partial\nu \equiv \mathrm{d}\nu/\mathrm{d}\rho$ and $\partial\Gamma \equiv \mathrm{d}\Gamma/\mathrm{d}\rho$, and

$$\zeta_\| \equiv -\mu[\bar\rho] + \bar g^2(\xi+\chi_2), \quad \zeta_\perp \equiv -\mu[\bar\rho] + \bar g^2(\xi-\chi_2), \quad \kappa_\pm \equiv 2\kappa_1[\bar\rho] \pm \kappa_2[\bar\rho], \quad \lambda_\pm \equiv \lambda_4 \pm \lambda_3\,.$$

From the expressions of the hydrodynamic equation coefficients, we find that $\zeta_\|$ and $\zeta_\perp$ are both positive, meaning that $\delta f_\|$ and $\delta f_\perp$ both relax on finite timescales and are thus non-hydrodynamic. Similarly, $\delta g_\|$ is also non-hydrodynamic as we linearized the equations in the regime where $\nu[\bar\rho] > 0$. Furthermore, as $\tau_r$ can in principle be arbitrary large, allowing us to study the dynamics of perturbations on time and length scales much smaller than that typically needed for the particles to reverse their orientation, for now we consider $\delta g_0$ as hydrodynamic and don't enslave it to the other modes.

To leading order, we thus find that over large enough timescales

$$\delta f_{\parallel} \simeq \zeta_{\parallel}^{-1}\left[\bar{g}\left(\partial\alpha-\chi_1\bar{g}^2\right)(1-\zeta_{\parallel}^{-1}\partial_t)\delta g_0-\frac{1}{2}\left(1-\frac{\kappa_+\bar{g}^2\left(\partial\nu-\partial\Gamma\bar{g}^2\right)}{\nu[\bar{\rho}]}\right)\partial_{\parallel}\delta\rho+\kappa_-\bar{g}\partial_{\perp}\delta g_{\perp}\right],$$

$$\delta f_{\perp} \simeq \zeta_{\perp}^{-1}\left[-\frac{1}{2}\left(1+\frac{\kappa_-\bar{g}^2\left(\partial\nu-\partial\Gamma\bar{g}^2\right)}{\nu[\bar{\rho}]}\right)\partial_{\perp}\delta\rho+\kappa_+\bar{g}\partial_{\parallel}\delta g_{\perp}\right],$$

$$\delta g_{\parallel} \simeq (2\nu[\bar{\rho}])^{-1}\left[\bar{g}\left(\partial\nu-\partial\Gamma\bar{g}^2\right)(1-(2\nu[\bar{\rho}])^{-1}\partial_t)\delta\rho-\frac{1}{2}\left(1+2\sigma\bar{g}^2-\frac{2\lambda_+\bar{g}^2\left(\partial\alpha-\chi_1\bar{g}^2\right)}{\zeta_{\parallel}}\right)\partial_{\parallel}\delta g_0\right].$$

Replacing these expressions in the equations of $\delta\rho$, $\delta g_0$ and $\delta g_{\perp}$, we finally get Eqs. (7) of the main text:

$$\partial_t\delta\rho=\left(D_{\rho\parallel}\partial^2_{\parallel\parallel}+D_{\rho\perp}\partial^2_{\perp\perp}\right)\delta\rho-\lambda_0\partial_{\parallel}\delta g_0+D_{\rho g}\partial^2_{\parallel\perp}\delta g_{\perp}+\eta_1\partial^2_{\parallel t}\delta g_0\,, \tag{21a}$$

$$\partial_t\delta g_0=\left(D_{0\parallel}\partial^2_{\parallel\parallel}-2\tau_r^{-1}\right)\delta g_0-\kappa_0\partial_{\parallel}\delta\rho-v_0\partial_{\perp}\delta g_{\perp}+\eta_2\partial^2_{\parallel t}\delta\rho\,, \tag{21b}$$

$$\partial_t\delta g_{\perp}=\left(D_{\parallel}\partial^2_{\parallel\parallel}+D_{\perp}\partial^2_{\perp\perp}\right)\delta g_{\perp}+\gamma\partial^2_{\parallel\perp}\delta\rho-\alpha_0\partial_{\perp}\delta g_0+\eta_3\partial^2_{\perp t}\delta g_0\,. \tag{21c}$$

with the bare coefficients

$$D_{\rho\parallel}\equiv\frac{1}{2\zeta_{\parallel}}\left(1-\frac{\kappa_+\bar{g}^2\left(\partial\nu-\partial\Gamma\bar{g}^2\right)}{\nu[\bar{\rho}]}\right),\quad D_{\rho\perp}\equiv\frac{1}{2\zeta_{\perp}}\left(1+\frac{\kappa_-\bar{g}^2\left(\partial\nu-\partial\Gamma\bar{g}^2\right)}{\nu[\bar{\rho}]}\right),$$

$$\lambda_0\equiv\frac{\bar{g}\left(\partial\alpha-\chi_1\bar{g}^2\right)}{\zeta_{\parallel}},\qquad D_{\rho g}\equiv-\frac{\kappa_+\bar{g}}{\zeta_{\perp}}-\frac{\kappa_-\bar{g}}{\zeta_{\parallel}},$$

$$\eta_1\equiv\frac{\bar{g}\left(\partial\alpha-\chi_1\bar{g}^2\right)}{\zeta_{\parallel}^2},\qquad D_{0\parallel}\equiv\frac{1}{4\nu[\bar{\rho}]}\left(1+2\sigma\bar{g}^2-\frac{2\lambda_+\bar{g}^2\left(\partial\alpha-\chi_1\bar{g}^2\right)}{\zeta_{\parallel}}\right),$$

$$\kappa_0\equiv\frac{\bar{g}\left(\partial\nu-\partial\Gamma\bar{g}^2\right)}{2\nu[\bar{\rho}]}\qquad v_0=1,$$

$$\eta_2\equiv\frac{\bar{g}\left(\partial\nu-\partial\Gamma\bar{g}^2\right)}{4\nu^2[\bar{\rho}]}\qquad D_{\parallel}\equiv\Omega[\bar{\rho}]+\frac{\lambda_+\kappa_+\bar{g}^2}{\zeta_{\perp}},$$

$$D_{\perp}\equiv\Omega[\bar{\rho}]-\frac{\lambda_-\kappa_-\bar{g}^2}{\zeta_{\parallel}},\qquad \gamma\equiv-\frac{\lambda_+\bar{g}}{2\zeta_{\perp}}\left(1+\frac{\kappa_-\bar{g}^2\left(\partial\nu-\partial\Gamma\bar{g}^2\right)}{\nu[\bar{\rho}]}\right)+-\frac{\lambda_-\bar{g}}{2\zeta_{\parallel}}\left(1-\frac{\kappa_+\bar{g}^2\left(\partial\nu-\partial\Gamma\bar{g}^2\right)}{\nu[\bar{\rho}]}\right),$$

$$\alpha_0\equiv\frac{1}{2}-\sigma\bar{g}^2+\frac{\lambda_-\bar{g}^2\left(\partial\alpha-\chi_1\bar{g}^2\right)}{\zeta_{\parallel}},\qquad \eta_3\equiv\frac{\lambda_-\bar{g}^2\left(\partial\alpha-\chi_1\bar{g}^2\right)}{\zeta_{\parallel}^2}.$$

**The small $\tau_r$ regime**

Before proceeding further, we now show that in the small $\tau_r$ limit Eqs. (21) reduce to the linear equations usually considered to describe the fluctuating phase of dry active nematics [4, 8, 9]. If we take $\tau_r$ small enough such that we observe the dynamics of fluctuations on time and lengthscales on which the particles typically reverse their orientations many times, then $\delta g_0$ becomes non-hydrodynamic, leading to

$$\delta g_0\simeq-\frac{\tau_r}{2}\left(\kappa_0\partial_{\parallel}\delta\rho+v_0\partial_{\perp}\delta g_{\perp}\right),$$

such that replacing its occurrences in the equations for the density and transverse order fluctuations we get at second order in gradients

$$\partial_t\delta\rho=\left(\tilde{D}_{\rho\parallel}\partial^2_{\parallel\parallel}+D_{\rho\perp}\partial^2_{\perp\perp}\right)\delta\rho+\tilde{D}_{\rho g}\partial^2_{\parallel\perp}\delta g_{\perp}\,, \tag{22a}$$

$$\partial_t\delta g_{\perp}=\left(D_{\parallel}\partial^2_{\parallel\parallel}+\tilde{D}_{\perp}\partial^2_{\perp\perp}\right)\delta g_{\perp}+\tilde{\gamma}\partial^2_{\parallel\perp}\delta\rho\,. \tag{22b}$$

For $\delta g_{\perp}$ playing the role of the transverse fluctuations of the nematic order parameter, Eqs. (22) describe the evolution of linear perturbations around the homogeneous order of an active nematic.

**The limit $\tau_r \to +\infty$**

*Space-time correlation functions* In the limit where $\tau_r$ is very large, typically much larger than the observation time and $\ell_r = v_0\tau_r$ is much larger than the system size, we neglect the term $2\tau_r^{-1}\delta g_0$ in Eq. (21b). Moreover, to compute the space and time correlation functions of the three hydrodynamic fields $\delta\rho$, $\delta g_0$ and $\delta g_\perp$, we add to Eqs. (21a), (21b) and (21c) respectively the noise terms $\partial_\parallel h_{\rho\parallel} + \partial_\perp h_{\rho\perp}$, $h_0$ and $h_\perp$ which are all additive, uncorrelated, with zero mean, and satisfy

$$\left\langle \partial_\parallel h_{\rho\parallel}(\boldsymbol{r},t)\partial_\parallel h_{\rho\parallel}(\boldsymbol{r}',t')\right\rangle = \Delta_{\rho\parallel}\partial^2_{\parallel\parallel}\delta(\boldsymbol{r}-\boldsymbol{r}')\delta(t-t'), \quad \left\langle \partial_\perp h_{\rho\perp}(\boldsymbol{r},t)\partial_\perp h_{\rho\perp}(\boldsymbol{r}',t')\right\rangle = \Delta_{\rho\perp}\partial^2_{\perp\perp}\delta(\boldsymbol{r}-\boldsymbol{r}')\delta(t-t'),$$
$$\left\langle h_0(\boldsymbol{r},t)h_0(\boldsymbol{r}',t')\right\rangle = \Delta_0\delta(\boldsymbol{r}-\boldsymbol{r}')\delta(t-t'), \quad \left\langle h_\perp(\boldsymbol{r},t)h_\perp(\boldsymbol{r}',t')\right\rangle = \Delta_\perp\delta(\boldsymbol{r}-\boldsymbol{r}')\delta(t-t').$$

For completeness, we also consider a term $D_{0\perp}\partial^2_{\perp\perp}\delta g_0$ in the rhs of Eq. (21b) as it is allowed by the symmetries. Going into Fourier space, we thus need to solve the linear system

$$\begin{pmatrix} D_{\rho\parallel}q_\parallel^2 + D_{\rho\perp}q_\perp^2 - i\omega & i\lambda_0 q_\parallel - \eta_1\omega q_\parallel & D_{\rho g}q_\parallel q_\perp \\ i\kappa_0 q_\parallel - \eta_2\omega q_\parallel & D_{0\parallel}q_\parallel^2 + D_{0\perp}q_\perp^2 - i\omega & iv_0 q_\perp \\ \gamma q_\parallel q_\perp & i\alpha_0 q_\perp - \eta_3\omega q_\perp & D_\parallel q_\parallel^2 + D_\perp q_\perp^2 - i\omega \end{pmatrix}\begin{pmatrix}\delta\hat\rho(\omega,\boldsymbol{q})\\ \delta\hat g_0(\omega,\boldsymbol{q})\\ \delta\hat g_\perp(\omega,\boldsymbol{q})\end{pmatrix} = \begin{pmatrix} iq_\parallel\hat h_{\rho\parallel}(\omega,\boldsymbol{q}) + iq_\perp\hat h_{\rho\perp}(\omega,\boldsymbol{q})\\ \hat h_0(\omega,\boldsymbol{q})\\ \hat h_\perp(\omega,\boldsymbol{q})\end{pmatrix},$$

where the hats refer to variables expressed in Fourier space. The full solution of this system is generally tedious to calculate explicitly, and moreover not very instructive regarding the physics of the system. We thus consider the limit $\omega, q \to 0$, the matrix on the lhs is inverted using Mathematica (Wolfram Research, Champaign, IL, USA) and the resulting expressions of the modes are truncated up to second order in $q$ and $\omega$. Taking the square norm of the solution then leads to the following expressions of the correlation functions given in Eqs. (8) of the main text:

$$\left\langle|\delta\hat\rho(\omega,\boldsymbol{q})|^2\right\rangle \underset{\omega,q\to0}{\simeq} \frac{(q_\parallel^2\Delta_{\rho\parallel} + q_\perp^2\Delta_{\rho\perp})(\omega^2 - v_0\alpha_0 q_\perp^2)^2 + \Delta_0\lambda_0^2 q_\parallel^2\omega^2 + \Delta_\perp(v_0\lambda_0)^2 q_\parallel^2 q_\perp^2}{\mathcal{D}(\omega,\boldsymbol{q})}, \tag{23a}$$

$$\left\langle|\delta\hat g_0(\omega,\boldsymbol{q})|^2\right\rangle \underset{\omega,q\to0}{\simeq} \frac{(q_\parallel^2\Delta_{\rho\parallel} + q_\perp^2\Delta_{\rho\perp})\kappa_0^2 q_\parallel^2\omega^2 + \Delta_0\omega^4 + \Delta_\perp v_0^2 q_\perp^2\omega^2}{\mathcal{D}(\omega,\boldsymbol{q})}, \tag{23b}$$

$$\left\langle|\delta\hat g_\perp(\omega,\boldsymbol{q})|^2\right\rangle \underset{\omega,q\to0}{\simeq} \frac{(q_\parallel^2\Delta_{\rho\parallel} + q_\perp^2\Delta_{\rho\perp})(\alpha_0\kappa_0)^2 q_\parallel^2 q_\perp^2 + \Delta_0\alpha_0^2 q_\perp^2\omega^2 + \Delta_\perp(\omega^2 - \kappa_0\lambda_0 q_\parallel^2)^2}{\mathcal{D}(\omega,\boldsymbol{q})}, \tag{23c}$$

where we have defined

$$\mathcal{D}(\omega,\boldsymbol{q}) \equiv |\omega - i\varepsilon_{\rm d}(\boldsymbol{q})|^2 \times |\omega - c(\theta_{\boldsymbol{q}})q + i\varepsilon_{\rm p}(\boldsymbol{q})|^2 \times |\omega + c(\theta_{\boldsymbol{q}})q + i\varepsilon_{\rm p}(\boldsymbol{q})|^2. \tag{24}$$

where $\theta_{\boldsymbol{q}}$ denotes the angle between $\boldsymbol{q}$ and the mean order, and

$$c(\theta_{\boldsymbol{q}}) = \sqrt{\kappa_0\lambda_0\cos^2(\theta_{\boldsymbol{q}}) + v_0\alpha_0\sin^2(\theta_{\boldsymbol{q}})}, \tag{25a}$$

$$\varepsilon_{\rm d}(\boldsymbol{q}) = D_{\rho\perp}q_\perp^2 + \left(D_{\rho\parallel} - \frac{\kappa_0}{v_0}D_{\rho g} - \frac{\lambda_0}{\alpha_0}\gamma + \frac{\lambda_0\kappa_0}{v_0\alpha_0}(D_\perp - D_{\rho\perp})\right)q_\parallel^2 \sim q^2, \tag{25b}$$

$$\varepsilon_{\rm p}(\boldsymbol{q}) = \frac{1}{2}\left[(D_\perp + D_{0\perp} - v_0\eta_3)q_\perp^2 + \left(D_\parallel + D_{0\parallel} + \frac{\kappa_0}{v_0}D_{\rho g} + \frac{\lambda_0}{\alpha_0}\gamma - \kappa_0\eta_1 - \lambda_0\eta_2 - \frac{\lambda_0\kappa_0}{v_0\alpha_0}(D_\perp - D_{\rho\perp})\right)q_\parallel^2\right] \sim q^2. \tag{25c}$$

Eqs. (23) therefore predict that the space-time correlation functions represented as function of the frequencies $\omega$ generally exhibit three distinct peaks. The first one is diffusive since always centered at $\omega = 0$, while the two others reveal the existence of propagating sound modes in the zero-reversals nematic liquid. This situation is similar to that found in a Toner Tu liquid, albeit with some differences. Indeed, we find in our case that the two propagating modes travel in opposite directions (their dispersion relation obeys $\omega \simeq \pm c(\theta_{\boldsymbol{q}})q$), while this is not the case in polar systems [5] as the corresponding ordered phase possesses different symmetries.

Finally, the dampings of all modes are set by the $\varepsilon_{\rm d,p}$ coefficients, which all scale as $\sim q^2$ corresponding to diffusive damping. As we will show in the following, this scaling is generally affected by nonlinearities, while the sound modes speeds are not renormalized.

*Equal-time correlation functions* Equal-time correlation functions are obtained by integrating Eqs. (23) over $\omega$. After some calculations and using the fact that in the $\omega, q \to 0$ limit the space-time correlations are dominated by the three peaks of widths $\sim q^2$, we get:

$$\left\langle|\delta\hat\rho(\boldsymbol{q})|^2\right\rangle \underset{q\to0}{\simeq} \frac{(q_\parallel^2\Delta_{\rho\parallel} + q_\perp^2\Delta_{\rho\perp})\left(2(c^2(\theta_{\boldsymbol{q}})q^2 - q_\perp^2 v_0\alpha_0)^2 + (v_0\alpha_0)^2 q_\perp^4\right)}{c^4(\theta_{\boldsymbol{q}})q^6} + \frac{\Delta_0\lambda_0^2 q_\parallel^2}{c^2(\theta_{\boldsymbol{q}})q^4} + \frac{\Delta_\perp q_\parallel^2 q_\perp^2(v_0\lambda_0)^2}{c^4(\theta_{\boldsymbol{q}})q^6}, \tag{26a}$$

$$\left\langle|\delta\hat{g}_0(\boldsymbol{q})|^2\right\rangle \underset{q\to 0}{\simeq} \frac{(q_\parallel^2\Delta_{\rho\parallel}+q_\perp^2\Delta_{\rho\perp})\kappa_0^2q_\parallel^2}{c^2(\theta_{\boldsymbol{q}})q^4}+\frac{\Delta_0}{q^2}+\frac{\Delta_\perp q_\perp^2 v_0^2}{c^2(\theta_{\boldsymbol{q}})q^4}\,, \tag{26b}$$

$$\left\langle|\delta\hat{g}_\perp(\boldsymbol{q})|^2\right\rangle \underset{q\to 0}{\simeq} \frac{(q_\parallel^2\Delta_{\rho\parallel}+q_\perp^2\Delta_{\rho\perp})(\alpha_0\kappa_0)^2q_\parallel^2q_\perp^2}{c^4(\theta_{\boldsymbol{q}})q^6}+\frac{\Delta_0\alpha_0^2q_\perp^2}{c^2(\theta_{\boldsymbol{q}})q^4}+\frac{\Delta_\perp\left(2(c^2(\theta_{\boldsymbol{q}})q^2-q_\parallel^2\kappa_0\lambda_0)^2+(\kappa_0\lambda_0)^2q_\parallel^4\right)}{c^4(\theta_{\boldsymbol{q}})q^6}\,, \tag{26c}$$

From these expressions, we read that all equal-time correlations diverge in almost all directions of space as $q^{-2}$ in the limit $q\to 0$. Such behavior implies a logarithmic divergence of order fluctuations in two dimensions, and thus quasi-long-range order at odds with the numerical data presented in the main text and in Ref. [10]. From the similarities between Eqs. (18) and the Toner Tu equations, we nevertheless expect the linearized hydrodynamics to break down in low dimensions, such that, as we will show later, the existence of long-range order is cannot be excluded. We moreover note that $\langle|\delta\hat{\rho}(\boldsymbol{q})|^2\rangle \sim q^{-2}$ implies the presence of giant number fluctuations (GNF) (the variance of the particle number in sub-systems scales faster than its mean) in the homogeneous nematic phase, in agreement with numerical simulations results [10] and the overall phenomenology of dry aligning dilute active matter [3, 6]. The corresponding GNF exponent is expected to be renormalized by nonlinearities as well.

From Eqs. (26) taking respectively $q_\perp=0$ and $q_\parallel=0$, we deduce the following scalings of the correlation in the directions longitudinal and transverse to the global order:

$$\left\langle|\delta\hat{\rho}(q_\parallel)|^2\right\rangle \underset{q_\parallel\to 0}{\simeq} \Delta_{\rho\parallel}\times\text{const}+\frac{\Delta_0\lambda_0}{\kappa_0q_\parallel^2},\qquad \left\langle|\delta\hat{\rho}(q_\perp)|^2\right\rangle \underset{q_\perp\to 0}{\simeq} \Delta_{\rho\perp}\times\text{const}, \tag{27a}$$

$$\left\langle|\delta\hat{g}_0(q_\parallel)|^2\right\rangle \underset{q_\parallel\to 0}{\simeq} \Delta_{\rho\parallel}\times\text{const}+\frac{\Delta_0}{q_\parallel^2},\qquad \left\langle|\delta\hat{g}_0(q_\perp)|^2\right\rangle \underset{q_\perp\to 0}{\simeq} \frac{\Delta_0}{q_\perp^2}+\frac{\Delta_\perp v_0}{\alpha_0q_\perp^2}, \tag{27b}$$

$$\left\langle|\delta\hat{g}_\perp(q_\parallel)|^2\right\rangle \underset{q_\parallel\to 0}{\simeq} \frac{\Delta_\perp}{q_\parallel^2},\qquad \left\langle|\delta\hat{g}_\perp(q_\perp)|^2\right\rangle \underset{q_\perp\to 0}{\simeq} \frac{\Delta_0\alpha_0}{v_0q_\perp^2}+\frac{\Delta_\perp}{q_\perp^2}. \tag{27c}$$

## SOME ELEMENTS OF THE NONLINEAR THEORY

As stated above, from the similarities between the hydrodynamic theory derived here and the Toner Tu equations we expect a breakdown of linearized hydrodynamics in dimensions low enough. This section is devoted to desmonstrate this prediction. The enslaving of the fast modes $\delta f_1$ and $\delta g_\parallel$ performed at the linear level can also be implemented keeping the leading order (in fields and gradients) nonlinearities of the hydrodynamic equations (18). The full nonlinear evolution equations for the perturbations around the ordered state read

$$\begin{aligned}
\partial_t\delta f_\parallel = {}& \mathcal{L}_{f_\parallel}+\partial\mu_1\delta\rho\delta f_\parallel+\left(\partial\alpha-\chi_1\bar{g}^2\right)\delta g_0\delta g_\parallel-(\xi+\chi_2)\left(2\bar{g}\delta g_\parallel+\delta g_\parallel^2\right)\delta f_\parallel-(\xi-\chi_2)\delta g_\perp^2\delta f_\parallel-2\chi_2\left(\bar{g}+\delta g_\parallel\right)\delta g_\perp\delta f_\perp\\
&-\chi_1\delta g_0\left(2\bar{g}\delta g_\parallel+\delta g_\parallel^2+\delta g_\perp^2\right)\left(\bar{g}+\delta g_\parallel\right)+D_2\delta g_0\Delta\delta g_\parallel+2\bar{g}\left(\partial\kappa_1+\partial\kappa_2\right)\delta\rho\partial_\parallel\delta g_\parallel+2\bar{g}\left(\partial\kappa_1-\partial\kappa_2\right)\delta\rho\partial_\perp\delta g_\perp\\
&+\left[2(\kappa_1+\partial\kappa_1\delta\rho)+\kappa_2+\partial\kappa_2\delta\rho\right]\left(\delta g_\parallel\partial_\parallel+\delta g_\perp\partial_\perp\right)\delta g_\parallel+\left[2(\kappa_1+\partial\kappa_1\delta\rho)-\kappa_2-\partial\kappa_2\delta\rho\right]\left(\delta g_\parallel\partial_\perp-\delta g_\perp\partial_\parallel\right)\delta g_\perp\\
&+\kappa_3\left[\left(\partial_\parallel\delta g_\parallel-\partial_\perp\delta g_\perp\right)\partial_\parallel+\left(\partial_\parallel\delta g_\perp+\partial_\perp\delta g_\parallel\right)\partial_\perp\right]\delta g_0
\end{aligned} \tag{28a}$$

$$\begin{aligned}
\partial_t\delta f_\perp = {}& \mathcal{L}_{f_\perp}+\partial\mu_1\delta\rho\delta f_\perp+\left(\partial\alpha-\chi_1\bar{g}^2\right)\delta g_0\delta g_\perp-(\xi-\chi_2)\left(2\bar{g}\delta g_\parallel+\delta g_\parallel^2\right)\delta f_\perp-(\xi+\chi_2)\delta g_\perp^2\delta f_\parallel-2\chi_2\left(\bar{g}+\delta g_\parallel\right)\delta g_\perp\delta f_\parallel\\
&-\chi_1\delta g_0\left(2\bar{g}\delta g_\parallel+\delta g_\parallel^2+\delta g_\perp^2\right)\delta g_\perp+D_2\delta g_0\Delta\delta g_\perp+2\bar{g}\left(\partial\kappa_1+\partial\kappa_2\right)\delta\rho\partial_\parallel\delta g_\perp-2\bar{g}\left(\partial\kappa_1-\partial\kappa_2\right)\delta\rho\partial_\perp\delta g_\parallel\\
&+\left[2(\kappa_1+\partial\kappa_1\delta\rho)+\kappa_2+\partial\kappa_2\delta\rho\right]\left(\delta g_\parallel\partial_\parallel+\delta g_\perp\partial_\perp\right)\delta g_\perp-\left[2(\kappa_1+\partial\kappa_1\delta\rho)-\kappa_2-\partial\kappa_2\delta\rho\right]\left(\delta g_\parallel\partial_\perp-\delta g_\perp\partial_\parallel\right)\delta g_\parallel\\
&+\kappa_3\left[\left(\partial_\parallel\delta g_\perp+\partial_\perp\delta g_\parallel\right)\partial_\parallel-\left(\partial_\parallel\delta g_\parallel-\partial_\perp\delta g_\perp\right)\partial_\perp\right]\delta g_0
\end{aligned} \tag{28b}$$

$$\begin{aligned}
\partial_t\delta g_\parallel = {}& \mathcal{L}_{g_\parallel}-\sigma\left[\left(2\bar{g}\delta g_\parallel+\delta g_\parallel^2-\delta g_\perp^2\right)\partial_\parallel+2\left(\bar{g}+\delta g_\parallel\right)\delta g_\perp\partial_\perp\right]\delta g_0+\left(\partial\nu_1-\partial\Gamma\bar{g}^2\right)\delta\rho\delta g_\parallel\\
&-2\bar{g}\delta g_\parallel\left(\Gamma\delta g_\parallel+\partial\Gamma\delta\rho(\bar{g}+\delta g_\parallel)\right)-\left(\Gamma+\partial\Gamma\delta\rho\right)\left(\delta g_\parallel^2+\delta g_\perp^2\right)(\bar{g}+\delta g_\parallel)+\partial\beta\delta g_0\delta f_\parallel+\partial\Omega\delta\rho\Delta\delta g_\parallel\\
&+(\lambda_1+\lambda_2)\left(\delta f_\parallel\partial_\parallel\delta g_\parallel+\delta f_\perp\partial_\perp\delta g_\parallel\right)+(\lambda_1-\lambda_2)\left(\delta f_\parallel\partial_\perp\delta g_\perp-\delta f_\perp\partial_\parallel\delta g_\perp\right)+(\lambda_1+\lambda_3)\left(\delta g_\parallel\partial_\parallel\delta f_\parallel-\delta g_\perp\partial_\parallel\delta f_\perp\right)\\
&+(\lambda_1-\lambda_3)\left(\delta g_\perp\partial_\perp\delta f_\parallel+\delta g_\parallel\partial_\perp\delta f_\perp\right)+\delta g_0(2\lambda_4+\lambda_5)\left((\bar{g}+\delta g_\parallel)\partial_\parallel+\delta g_\perp\partial_\perp\right)\delta g_\parallel\\
&+\delta g_0(2\lambda_4-\lambda_5)\left((\bar{g}+\delta g_\parallel)\partial_\perp-\delta g_\perp\partial_\parallel\right)\delta g_\perp\,,
\end{aligned} \tag{28c}$$

$$\partial_t\delta g_\perp = \mathcal{L}_{g_\perp}-\sigma\left[2\left(\bar{g}+\delta g_\parallel\right)\delta g_\perp\partial_\parallel-\left(2\bar{g}\delta g_\parallel+\delta g_\parallel^2-\delta g_\perp^2\right)\partial_\perp\right]\delta g_0+\left(\partial\nu_1-\partial\Gamma\bar{g}^2\right)\delta\rho\delta g_\perp$$

$$
\begin{aligned}
&- (\Gamma + \partial\Gamma\delta\rho)\left(2\bar{g}\delta g_{\|} + \delta g_{\|}^2 + \delta g_{\perp}^2\right)\delta g_{\perp} + \partial\beta\delta g_0\delta f_{\perp} + \partial\Omega\delta\rho\Delta\delta g_{\perp} + (\lambda_1+\lambda_2)\left(\delta f_{\|}\partial_{\|}\delta g_{\perp} + \delta f_{\perp}\partial_{\perp}\delta g_{\perp}\right)\\
&+ (\lambda_1-\lambda_2)\left(\delta f_{\perp}\partial_{\|}\delta g_{\|} - \delta f_{\|}\partial_{\perp}\delta g_{\|}\right) + (\lambda_1+\lambda_3)\left(\delta g_{\perp}\partial_{\|}\delta f_{\|} + \delta g_{\|}\partial_{\|}\delta f_{\perp}\right) + (\lambda_1-\lambda_3)\left(\delta g_{\perp}\partial_{\perp}\delta f_{\perp} - \delta g_{\|}\partial_{\perp}\delta f_{\|}\right)\\
&+ \delta g_0\left[(2\lambda_4+\lambda_5)\left((\bar{g}+\delta g_{\|})\partial_{\|} + \delta g_{\perp}\partial_{\perp}\right)\delta g_{\perp} + (2\lambda_4-\lambda_5)\left(\delta g_{\perp}\partial_{\|} - (\bar{g}+\delta g_{\|})\partial_{\perp}\right)\delta g_{\|}\right] , \qquad (28d)
\end{aligned}
$$

Where the operators $\mathcal{L}$ refer to the linear contributions to these equations and are given in Eqs. (20). Eqs. (28) obviously contain many nonlinearities, but only a restricted number of them are of interest to us. Using the similarities between Eqs. (18) and the Toner and Tu equations, we truncate the above equations up to order three in fields and gradients. With the above counting, all contributions from $\delta f_{\|}$, $\delta f_{\perp}$ and $\delta g_{\|}$ to $\delta\rho$, $\delta g_0$ and $\delta g_{\perp}$'s equations are at least of order two (including those coming from the linear terms), therefore we carry out the enslaving keeping at most terms of order two:

$$
\begin{aligned}
\delta f_{\|} &\simeq a_{\|}^1\delta g_0 + a_{\|}^2\partial_t\delta g_0 + a_{\|}^3\partial_{\|}\delta\rho + a_{\|}^4\partial_{\perp}\delta g_{\perp} + a_{\|}^5\delta\rho\delta g_0 ,\\
\delta f_{\perp} &\simeq a_{\perp}^1\partial_{\perp}\delta\rho + a_{\perp}^2\partial_{\|}\delta g_{\perp} + a_{\perp}^3\delta g_0\delta g_{\perp} ,\\
\delta g_{\|} &\simeq b_{\|}^1\delta\rho + b_{\|}^2\partial_t\delta\rho + b_{\|}^3\partial_{\|}\delta g_0 + b_{\|}^4\delta\rho^2 + b_{\|}^5\delta g_{\perp}^2 + b_{\|}^6\delta g_0^2 ,
\end{aligned}
$$

where we don't specify the expression of the coefficients as they are unimportant for the following discussion. After replacing these expressions, we get the following closed nonlinear equations given in the main text

$$
\begin{aligned}
\partial_t\delta\rho &= \left(D_{\rho\|}\partial_{\|\|}^2 + D_{\rho\perp}\partial_{\perp\perp}^2\right)\delta\rho - \lambda_0\partial_{\|}\delta g_0 + D_{\rho g}\partial_{\|\perp}^2\delta g_{\perp} + \eta_1\partial_{\|t}^2\delta g_0\\
&\quad + j_1\partial_{\|}\left(\delta g_0\delta\rho\right) + j_2\partial_{\perp}\left(\delta g_0\delta g_{\perp}\right) + \partial_{\|}h_{\rho\|} + \partial_{\perp}h_{\rho\perp} , \qquad (29a)\\
\partial_t\delta g_0 &= \left(D_{0\|}\partial_{\|\|}^2 + D_{0\perp}\partial_{\perp\perp}^2\right)\delta g_0 - \kappa_0\partial_{\|}\delta\rho - v_0\partial_{\perp}\delta g_{\perp} + \eta_2\partial_{\|t}^2\delta\rho + c_1\partial_{\|}\delta\rho^2 + c_2\partial_{\|}\delta g_{\perp}^2 + c_3\partial_{\|}\delta g_0^2 + h_0 , \qquad (29b)\\
\partial_t\delta g_{\perp} &= \left(D_{\|}\partial_{\|\|}^2 + D_{\perp}\partial_{\perp\perp}^2\right)\delta g_{\perp} + \gamma\partial_{\|\perp}^2\delta\rho - \alpha_0\partial_{\perp}\delta g_0 + \eta_3\partial_{\perp t}^2\delta g_0\\
&\quad + w_1\delta g_{\perp}\partial_{\|}\delta g_0 + w_2\delta g_0\partial_{\|}\delta g_{\perp} + w_3\delta g_0\partial_{\perp}\delta\rho + w_4\delta\rho\partial_{\perp}\delta g_0 + w_5\delta g_{\perp}\partial_t\delta\rho + h_{\perp} . \qquad (29c)
\end{aligned}
$$

Following standard procedures, we now perform the rescaling

$$
x_{\perp} \to b x_{\perp}, \quad x_{\|} \to b^{\xi}x_{\|}, \quad t \to b^z t, \quad \delta g_{\perp} \to b^{\chi}\delta g_{\perp}, \quad \delta g_0 \to b^{\chi_0}\delta g_0, \quad \delta\rho \to b^{\chi_\rho}\delta\rho .
$$

The exponent $\xi$ sets the anisotropy of the fluctuations scaling, $\xi = 1$ corresponding to an isotropic scaling. $z$ is the dynamical exponent, and as we will show later sets the damping of sound modes. Finally, the roughness exponents $\chi$, $\chi_0$ and $\chi_\rho$ set the scaling of fluctuations with distance. At the linear fixed point, all coefficients renormalize according to

$$
\begin{aligned}
&D_{\rho\|} \to b^{z-2\xi}D_{\rho\|}, && D_{\rho\perp} \to b^{z-2}D_{\rho\perp}, && D_{\rho g} \to b^{z+\chi-\chi_\rho-1-\xi}D_{\rho g}, && \lambda_0 \to b^{z+\chi_0-\chi_\rho-\xi}\lambda_0,\\
&\eta_1 \to b^{\chi_0-\chi_\rho-\xi}, && j_1 \to b^{z-\xi+\chi_0}j_1, && j_2 \to b^{z+\chi+\chi_0-\chi_\rho-1}j_2, && \Delta_{\rho\|} \to b^{z-2\chi_\rho-(d-1)-3\xi}\Delta_{\rho\|},\\
&\Delta_{\rho\perp} \to b^{z-2\chi_\rho-d-1-\xi}\Delta_{\rho\perp}, &&&&&&\\
&D_{0\|} \to b^{z-2\xi}D_{0\|}, && D_{0\perp} \to b^{z-2}D_{0\perp}, && \kappa_0 \to b^{z+\chi_\rho-\chi_0-\xi}\kappa_0, && v_0 \to b^{z+\chi-\chi_0-1}v_0,\\
&\eta_2 \to b^{\chi_\rho-\chi_0-\xi}\eta_2, && c_1 \to b^{z+2\chi_\rho-\chi_0-\xi}c_1, && c_2 \to b^{z+2\chi-\chi_0-\xi}c_2, && c_3 \to b^{z+\chi_0-\xi}c_3,\\
&\Delta_0 \to b^{z-2\chi_0-(d-1)-\xi}\Delta_0, &&&&&&\\
&D_{\|} \to b^{z-2\xi}D_{\|}, && D_{\perp} \to b^{z-2}D_{\perp}, && \gamma \to b^{z+\chi_\rho-\chi-1-\xi}\gamma, && \alpha_0 \to b^{z+\chi_0-\chi-1}\alpha_0,\\
&\eta_3 \to b^{\chi_0-\chi-1}\eta_3, && w_{1,2} \to b^{z+\chi_0-\xi}w_{1,2}, && w_{3,4} \to b^{z+\chi_0+\chi_\rho-\chi-1}w_{3,4}, && w_5 \to b^{\chi_\rho}w_5,\\
&\Delta_{\perp} \to b^{z-2\chi-(d-1)-\xi}\Delta_{\perp}, &&&&&&
\end{aligned}
$$

where, although Eqs. (29) have formally been derived in $d = 2$, their structure should remain similar in higher dimensions such that we reintroduce an arbitrary dimension $d$ for power counting.

The values of the exponents $\xi$, $z$, $\chi$, $\chi_\rho$ and $\chi_0$ at the linear fixed point are those that keep the amplitude of the fluctuations given by Eqs. (26) only fixed by lengthscales ($q$). To achieve this, we keep the diffusion constants, as well as the noise variances fixed, which leads to the following relations

$$
z-2=0, \quad z-2\xi=0, \quad z-2\chi-(d-1)-\xi=0, \quad z-2\chi_\rho-(d-1)-\xi=0, \quad z-2\chi_0-(d-1)-\xi=0 .
$$

Hence, after solving them we get the mean field exponents

$$z_{\rm lin} = 2, \quad \xi_{\rm lin} = 1, \quad \chi_{\rm lin} = \chi_{0,{\rm lin}} = \chi_{\rho,{\rm lin}} = 1 - \frac{d}{2}\,, \tag{30}$$

such that, in agreement with Eqs. (23) and (26) above, the linear theory indeed predicts an isotropic ($\xi = 1$), and diffusive ($z = 2$) scaling, with quasi-long-range order in $d = 2$ ($\chi_{\rm lin} = 0$). Note that the exponents (30) are identical to that of the linear Toner Tu and usual active nematics theories [5, 9].

Using the linear exponent (30), we find that except for $w_5$ all nonlinearities of Eqs. (29) are relevant in $d \leq d_c \equiv 4$, namely

$$j_{1,2} \to b^{\frac{4-d}{2}} j_{1,2}, \quad c_{1,2,3} \to b^{\frac{4-d}{2}} c_{1,2,3}, \quad w_{1,2,3,4} \to b^{\frac{4-d}{2}} w_{1,2,3,4}. \tag{31}$$

Therefore, most of nonlinearities in Eqs. (29) grow on large enough time and length scales ($b \to \infty$), such that the linear theory breaks down in $d \leq 4$.

Given the number of relevant nonlinearities, even a perturbative calculation of the exponents, which would moreover not teach us much about their $d = 2$ value, would be challenging. Nevertheless, we can conjecture the scaling of correlation functions in the nonlinear theory following existing results for the polar case [5]. Indeed, as motivated in the main text we expect the relations $\chi = \chi_0 = \chi_\rho$ to hold even at the nonlinear level, while the structure of Eqs. (29) and the correlation functions implies that the scaling of the later in the nonlinear theory is obtained using the renormalized coefficients and dampings

$$\tilde{\Delta} = q_\perp^{z-\zeta} f_\Delta\left(\frac{q_\parallel}{q_\perp^\xi}\right), \qquad \tilde{\varepsilon}_{\rm d,p} = q_\perp^z f_{\rm d,p}\left(\frac{q_\parallel}{q_\perp^\xi}\right), \tag{32}$$

while the speed $c(\theta_{\boldsymbol{q}})$ remains unchanged. Here we have defined the exponent $\zeta \equiv d - 1 + 2\chi + \xi$. The functions $f_\Delta$ and $f_i$ are unknown but are universal for polar flocks, and should satisfy

$$f_\Delta(x) \underset{x\to 0}{\to} \text{const}, \qquad f_\Delta(x) \underset{x\to\infty}{\to} x^{\frac{z-\zeta}{\xi}}, \qquad f_{\rm d,p}(x) \underset{x\to 0}{\to} \text{const}, \qquad f_{\rm d,p}(x) \underset{x\to\infty}{\to} x^{\frac{z}{\xi}}.$$

Using these rescalings, the equal time correlation functions should obey at the nonlinear level

$$\left\langle |\delta\hat{\rho}(\boldsymbol{q})|^2 \right\rangle \underset{q\to 0}{\simeq} q_\perp^{-\zeta} f_\rho\left(\frac{q_\parallel}{q_\perp^\xi}\right)\left[\cos^2(\theta_{\boldsymbol{q}}) K_\rho(\theta_{\boldsymbol{q}}) + q^2 L_\rho(\theta_{\boldsymbol{q}})\right], \tag{33a}$$

$$\left\langle |\delta\hat{g}_0(\boldsymbol{q})|^2 \right\rangle \underset{q\to 0}{\simeq} q_\perp^{-\zeta} f_0\left(\frac{q_\parallel}{q_\perp^\xi}\right)\left[K_0(\theta_{\boldsymbol{q}}) + q^2 L_0(\theta_{\boldsymbol{q}})\right], \tag{33b}$$

$$\left\langle |\delta\hat{g}_\perp(\boldsymbol{q})|^2 \right\rangle \underset{q\to 0}{\simeq} q_\perp^{-\zeta} f_\perp\left(\frac{q_\parallel}{q_\perp^\xi}\right)\left[K_\perp(\theta_{\boldsymbol{q}}) + q^2 \cos^2(\theta_{\boldsymbol{q}})\sin^2(\theta_{\boldsymbol{q}}) L_\perp(\theta_{\boldsymbol{q}})\right], \tag{33c}$$

where the $K_{\rho,0,\perp}$ and $L_{\rho,0,\perp}$ functions are positive and $\mathcal{O}(1)$, while the scaling functions $f_{\rho,0,\perp}$ satisfy $f_{\rho,0,\perp}(x) \underset{x\to 0}{\to}$ const and $f_{\rho,0,\perp}(x) \underset{x\to\infty}{\to} x^{-\zeta/\xi}$. Using the linear exponents (30), one can indeed check that these expressions correspond to (26). Finally, we deduce the following expressions of the equal-time correlation functions in the longitudinal and transverse directions:

$$\left\langle \left|\delta\hat{\rho}(q_\parallel)\right|^2 \right\rangle \underset{q_\parallel\to 0}{\sim} q_\parallel^{-\zeta/\xi}, \qquad \left\langle \left|\delta\hat{\rho}(q_\perp)\right|^2 \right\rangle \underset{q_\perp\to 0}{\sim} q_\perp^{2-\zeta},$$

$$\left\langle \left|\delta\hat{g}_0(q_\parallel)\right|^2 \right\rangle \underset{q_\parallel\to 0}{\sim} q_\parallel^{-\zeta/\xi}, \qquad \left\langle \left|\delta\hat{g}_0(q_\perp)\right|^2 \right\rangle \underset{q_\perp\to 0}{\sim} q_\perp^{-\zeta},$$

$$\left\langle \left|\delta\hat{g}_\perp(q_\parallel)\right|^2 \right\rangle \underset{q_\parallel\to 0}{\sim} q_\parallel^{-\zeta/\xi}, \qquad \left\langle \left|\delta\hat{g}_\perp(q_\perp)\right|^2 \right\rangle \underset{q_\perp\to 0}{\sim} q_\perp^{-\zeta}.$$

## SCALING OF THE GLOBAL ORDER PARAMETER

It is shown in the main text that in the long-range ordered phase the nematic order $S$ parameter scales with system size $L$ as $S(L) - S(\infty) \sim L^{-\varpi}$, where the exponent $\varpi$ is argued to be equal to $-2\chi/\xi$. Here, we demonstrate this result.

We denote $q(\boldsymbol{r},t) \equiv S_\infty + \delta Q_\parallel(\boldsymbol{r},t) + i\delta Q_\perp(\boldsymbol{r},t)$ the complex representation of 2 dimensional coarse grained nematic order, written as a uniform mean order $Q_\infty$ plus a fluctuating part. Denoting $s(t) = |\langle e^{i2\theta_k^t}\rangle_k|$ the instantaneous order parameter, it is expressed as function of $q$ as

$$s(t) = \frac{1}{L^2}\left|\int \mathrm{d}\boldsymbol{r}\, q(\boldsymbol{r},t)\right| = \left|S_\infty + \frac{1}{L^2}\int \mathrm{d}\boldsymbol{r}\, \left[\delta Q_\parallel(\boldsymbol{r},t) + i\delta Q_\perp(\boldsymbol{r},t)\right]\right|. \tag{34}$$

Recasting the norm as $|\cdot| = \sqrt{|\cdot|^2}$, we successively expand the square and the square root so as to obtain, at second order in fluctuations:

$$S(L) = S_\infty + \frac{1}{2L^4 S_\infty}\int \mathrm{d}\boldsymbol{r}\int \mathrm{d}\boldsymbol{r}'\langle \delta Q_\perp(\boldsymbol{r},t)\delta Q_\perp(\boldsymbol{r}',t)\rangle, \tag{35}$$

which relates the average global order parameter with the two-point equal time correlation function of $\delta Q_\perp$. Denoting $\boldsymbol{r}' - \boldsymbol{r} \equiv \boldsymbol{x}$, the latter is obtained from its expression in Fourier space (33c) at leading order in $q$ via

$$\begin{aligned}\langle \delta Q_\perp(\boldsymbol{r},t)\delta Q_\perp(\boldsymbol{r}+\boldsymbol{x},t)\rangle &\sim \int \mathrm{d}q_\parallel \mathrm{d}q_\perp e^{i(x_\parallel q_\parallel + x_\perp q_\perp)} q_\perp^{-\zeta} f_\perp\left(\frac{q_\parallel}{q_\perp^\xi}\right)\\ &\sim x_\perp^{2\chi}\int \mathrm{d}p_\parallel \mathrm{d}p_\perp e^{i\left(\frac{x_\parallel}{x_\perp^\xi}p_\parallel + p_\perp\right)} p_\perp^{-\zeta} f_\perp\left(\frac{p_\parallel}{p_\perp^\xi}\right)\\ &\equiv x_\perp^{2\chi}\mathcal{F}_\perp\left(\frac{x_\parallel}{x_\perp^\xi}\right),\end{aligned} \tag{36}$$

where to go from the first to the second line we have used the change of variables $p_\parallel \equiv x_\perp^\xi q_\parallel$ and $p_\perp \equiv x_\perp q_\perp$, while the function $\mathcal{F}_\perp$ satisfies asymptotically $\mathcal{F}_\perp(x) \underset{x\to 0}{\to}$ const and $\mathcal{F}_\perp(x) \underset{x\to\infty}{\to} x^{2\chi/\xi}$. As we measured $\xi > 1$ in the low noise phase of the nematic liquid, the scaling of the order correlation function is dominated on large scales by its contribution from the longitudinal direction ($x_\parallel \gg x_\perp^\xi$). Moreover, using that in finite systems the correlation length scales as $L$, we finally rewrite Eq. (35) as

$$S(L) - S_\infty \sim \frac{1}{2L^2 S_\infty}\int \mathrm{d}x\, x^{1+2\chi/\xi}\mathcal{G}\left(\frac{x}{L}\right) \sim L^{-\varpi}, \tag{37}$$

with $\varpi = -2\chi/\xi$, and where $\mathcal{G}$ is an unspecified finite size scaling function.


[1] B. Mahault, F. Ginelli, and H. Chaté, Phys. Rev. Lett. **123**, 218001 (2019).
[2] A. Peshkov, E. Bertin, F. Ginelli, and H. Chaté, Eur. Phys. J. Spec. Top. **223**, 1315 (2014).
[3] H. Chaté and B. Mahault, in *Active Matter and Non-Equilibrium Statistical Physics: A Synthetic and Self-Contained Overview*, edited by J. Tailleur (Oxford University Press, 2019) Chap. Dilute Dry Aligning Active Matter.
[4] E. Bertin, H. Chaté, F. Ginelli, S. Mishra, A. Peshkov, and S. Ramaswamy, New J. Phys. **15**, 085032 (2013).
[5] J. Toner, Phys. Rev. E **86**, 031918 (2012).
[6] H. Chaté, Annu. Rev. Cond. Matt. **11**, 189 (2020).
[7] L.-b. Cai, H. Chaté, Y.-q. Ma, and X.-q. Shi, Phys. Rev. E **99**, 010601 (2019).
[8] S. Mishra, R. A. Simha, and S. Ramaswamy, J. Stat. Mech. , P02003 (2010).
[9] S. Shankar, S. Ramaswamy, and M. C. Marchetti, Phys. Rev. E **97**, 012707 (2018).
[10] F. Ginelli, F. Peruani, M. Bär, and H. Chaté, Phys. Rev. Lett. **104**, 184502 (2010).
